# Supplementary material for: Fermi surface anisotropy in plasmonic metals increases the potential for efficient hot carrier extraction
Source: arXiv:2205.05007 source file (2022-12-09)
Supplement: Supplementary file 1 [file SI.pdf]

# Supplementary information for:
# 'Plasmonic hot carrier dynamics in directional conductors'

Sushant Kumar,[a] Christian Multunas,[b] and Ravishankar Sundararaman[ab*]

[a]Department of Materials Science & Engineering, 110 $8^{th}$ St, Troy, NY 12180, USA.
[b]Department of Physics, Applied Physics, and Astronomy, 110 $8^{th}$ St, Troy, NY 12180, USA.
*sundar@rpi.edu

Figures S1 and S2 respectively show the electronic and phonon band structures of each of the materials investigated in the main text. Additionally, the attached spreadsheet file in XLSX format includes key data for plots in the main text, including the spectral functions, relaxation times, dielectric functions and injection probabilities.

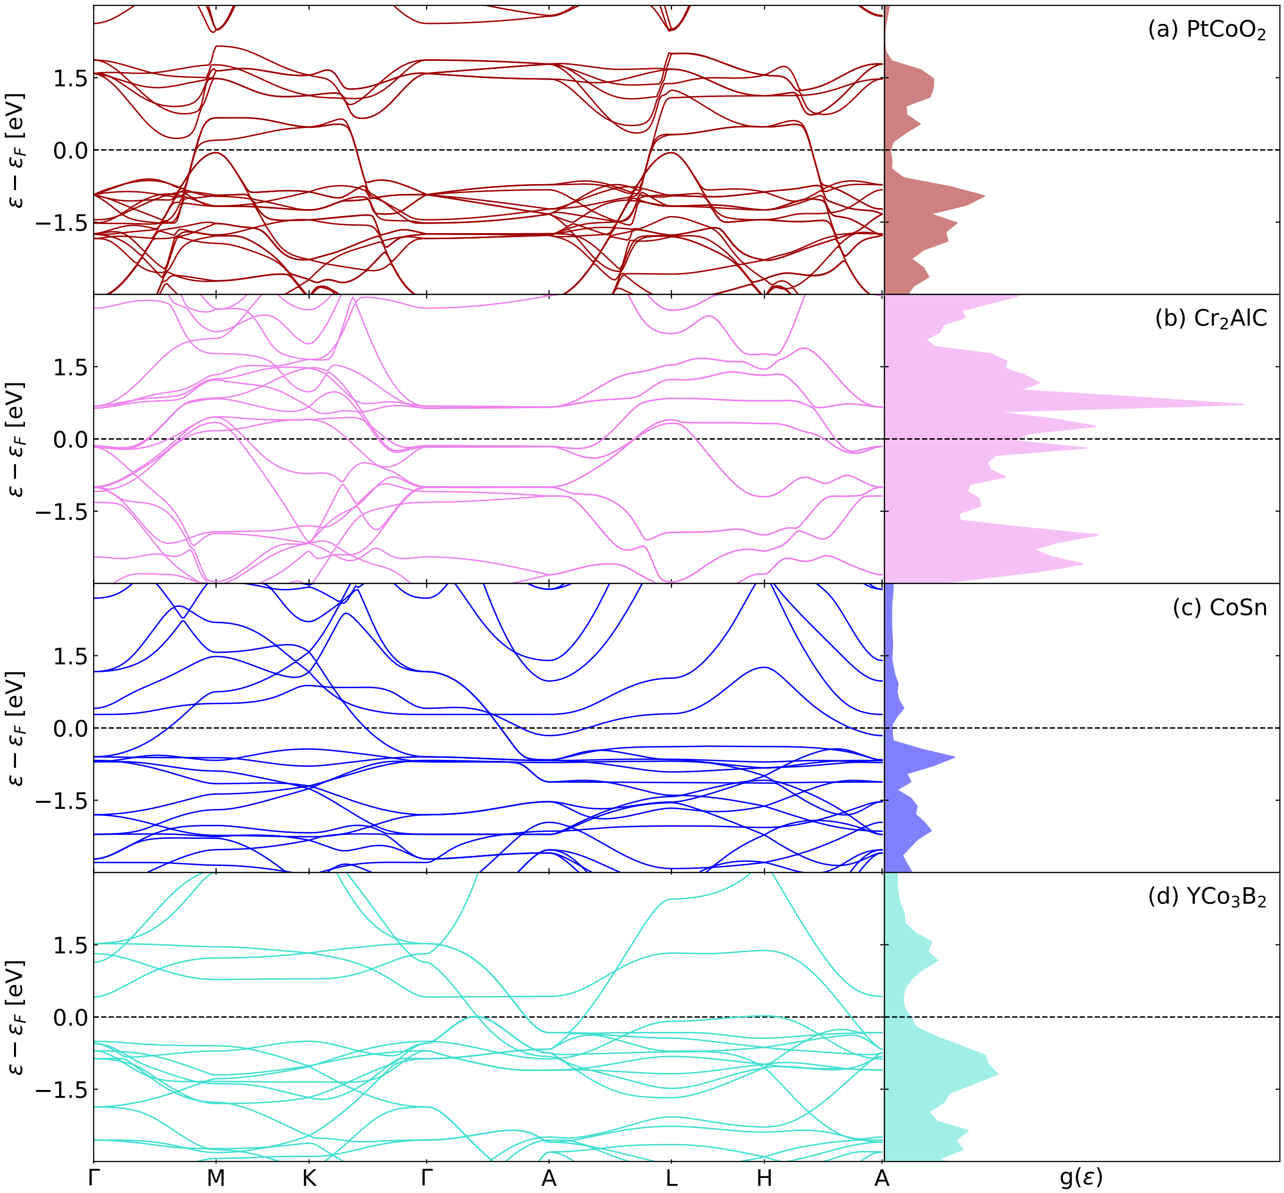


Figure S1: Electronic band structures of all four directional conductors investigated in the main text.

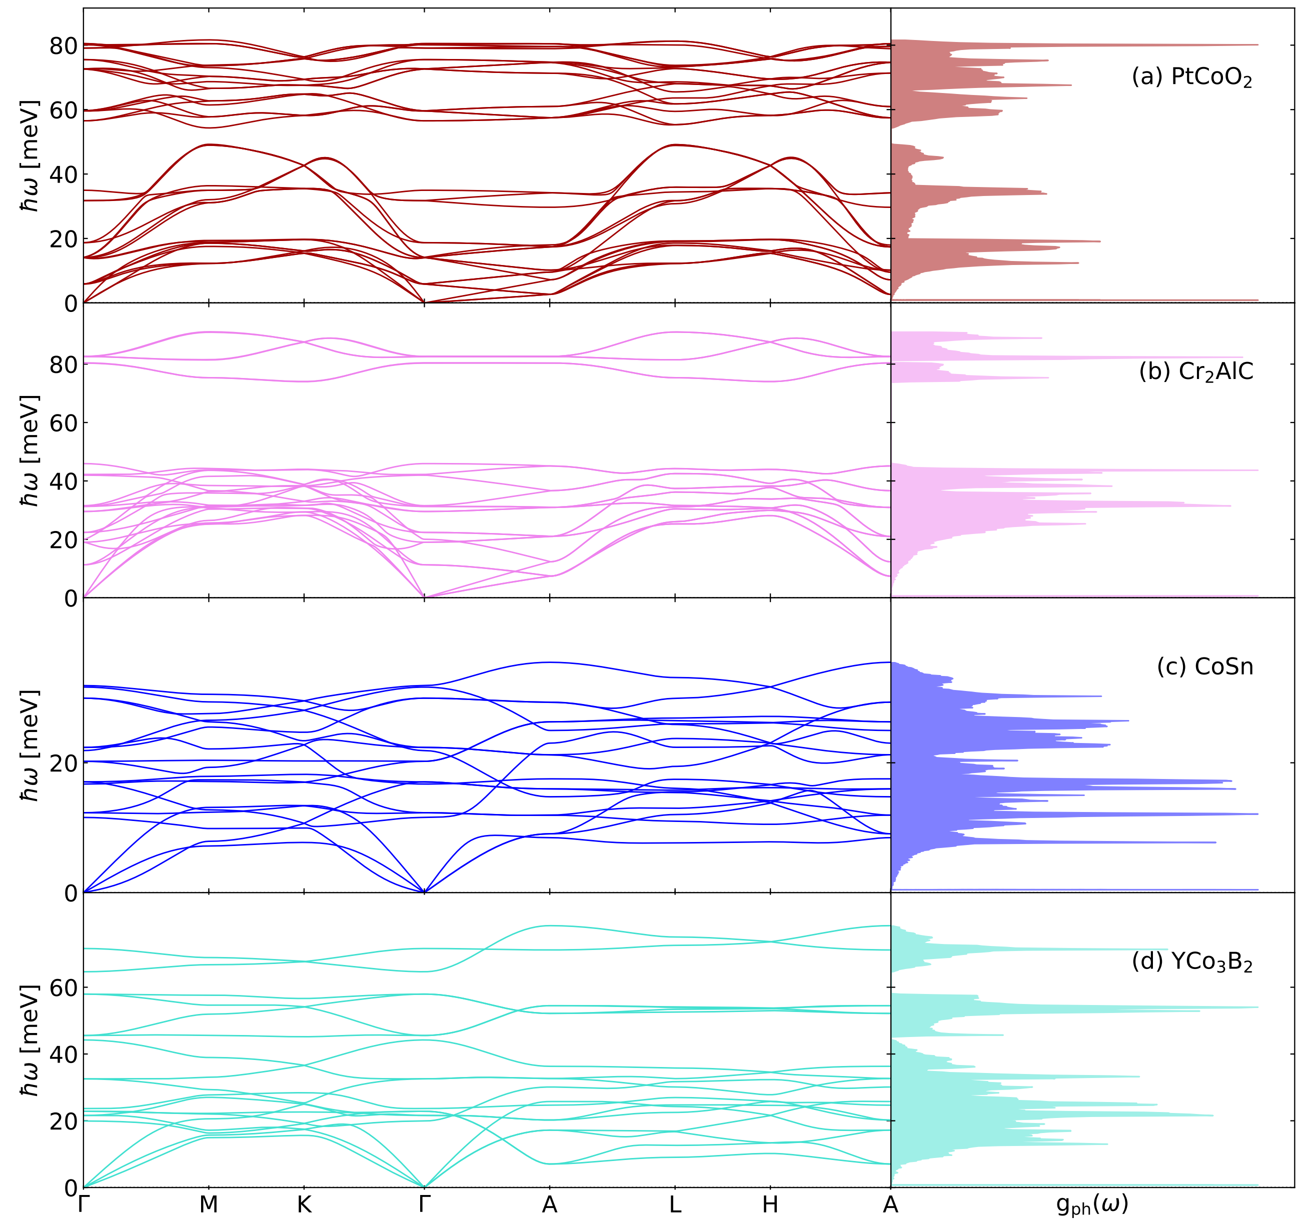


Figure S2: Phonon band structures of all four directional conductors investigated in the main text.
